# Supplementary material for: Token Highlighter: Inspecting and Mitigating Jailbreak Prompts for Large Language Models
Source: arXiv:2412.18171 source file (2024-12-25)
Supplement: Supplementary file 2 [file token_highlighter_alg.tex]

\subsection{Token Highlighter Algorithm}
\label{subapp:th_alg}
\input{pesudo_code/token_highlighter}
